# Supplementary material for: Finite-Cliquewidth Sets of Existential Rules: Toward a General Criterion for Decidable yet Highly Expressive Querying
Source: arXiv:2209.02464 source file (2022-09-06)
Supplement: Supplementary file 3 [file fo-well-decoration.tex]

\section{Definition of $\Phi_\mathrm{well}$ (\NoCaseChange{\cref{sec:cwdef}})}

Recall that a decorated tree $\mathcal{T}$ is called a \emph{well-decorated tree} \iffi
\begin{itemize}
\item for every null $s \in \{0,1\}^*$, $\mathcal{T}$ contains exactly one fact $\mathrm{Dec}(s)$ with  $\mathrm{Dec} \in \decorum$,
\item for every $\const{c}\in \mathrm{Cnst}$, $\mathcal{T}$ contains at most one fact of the form $\pred{c}_k(s)$,
%%%
%% THE FOLLOWING MODIFICATION WAS PLAIN WRONG AND HAS BEEN REVERTED -- DO NOT REINTRODUCE!!!
%%
%% \item for every null $s \in \{0,1\}^*$ and every $c\in \mathrm{Cnst}$, $\mathcal{T}$ contains at most one fact of the form $c_k(s)$;
%%
%% NOTE THAT CONSTANTS NEED TO BE UNIQUE ACROSS THE WHOLE MODEL!!!
%%%
\item if $\pred{Add}_{\rpred,\vk}(s) \in \mathcal{T}$ or $\pred{Recolor}_{k\to k'}(s) \in \mathcal{T}$,
       then $\pred{Void}(s0)\not\in \mathcal{T}$ and $\pred{Void}(s1) \in \mathcal{T}$,
\item if $\oplus(s) \in \mathcal{T}$, then $\pred{Void}(s0),\pred{Void}(s1) \not\in \mathcal{T}$,
\item if $\pred{Void}(s) \in \mathcal{T}$ or $\pred{c}_k(s) \in \mathcal{T}$, then  $\pred{Void}(s0),\pred{Void}(s1) \in \mathcal{T}$.
%\item if $\pred{Recolor}_{k\to k'}(s) \in \mathcal{T}$\!, $\pred{Add}_{\rpred,k,k'}(s) \in \mathcal{T}$\!, or $\pred{Add}_{\rpred,k}(s) \in \mathcal{T}$\!, then $\pred{Void}(s0)\not\in \mathcal{T}$ and $\pred{Void}(s1) \in \mathcal{T}$.

\end{itemize}

Here, fixing $\cols$, $\Sigma$, and $\mathrm{Cnst}$,  we will define a first-order sentence $\Phi_\mathrm{well}$ such that for any $(\cols,\mathrm{Cnst},\Sigma)$-decorated tree $\mathcal{T}$, $\mathcal{T}$ is well-decorated \ifandonlyif $\mathcal{T} \models \Phi_\mathrm{well}$. 

Let us denote $\decorum$ with $\Gamma$ and we write $\varphi^i_{\pred{Void}}(x)$ to abbreviate $\exists z (\pred{Succ}_i(x,z) \wedge \pred{Void}(z))$. 
Consider the following (where $\pred{c} \in \mathrm{Cnst}$, $\pred{d} \in \mathrm{Cnst} \cup\{\pred{*}\}$):
\begin{align*}
    \Phi^{\mathrm{funct}} &= \forall{x} \bigvee_{\mathrm{Dec} \in \Gamma}\Big( \mathrm{Dec}(x) \wedge \scaleobj{0.8}{\bigwedge_{\scaleobj{1.25}{\mathrm{Dec}' \in \Gamma \setminus \{\mathrm{Dec}\}}}} \neg\mathrm{Dec}'(x) \Big)\\ 
    \Phi^{\mathrm{unique}}_{\pred{c}_k} &=  \forall{xy}\; \pred{c}_k(x) \Rightarrow (\pred{c}_k(y) \Rightarrow x = y) \wedge \bigwedge_{k'\in \cols\setminus\{k\}}\neg\pred{c}_{k'}(y)\\
\end{align*}
\begin{align*}
    \Phi_{\pred{d}_k} &=  & \forall{x}\; \pred{d}_k(x) & \Rightarrow \ \ \varphi^0_{\pred{Void}}(x) \wedge \varphi^1_{\pred{Void}}(x)\\
    \Phi_{\pred{Add}_{\rpred,\vk}} &= & \forall{x}\; \pred{Add}_{\rpred,\vk}(x) & \Rightarrow \neg \varphi^0_{\pred{Void}}(x) \wedge \varphi^1_{\pred{Void}}(x)\\
    \Phi_{\pred{Recolor}_{k\to k'}} &= & \forall{x}\; \pred{Recolor}_{k\to k'}(x) & \Rightarrow \neg \varphi^0_{\pred{Void}}(x) \wedge \varphi^1_{\pred{Void}}(x)\\
    \Phi_{\oplus} &= & \forall{x}\; \oplus(x) & \Rightarrow \neg \varphi^0_{\pred{Void}}(x) \wedge \neg\varphi^1_{\pred{Void}}(x)\\
    \Phi_{\pred{Void}} &= &\forall{x}\; \pred{Void}(x) & \Rightarrow \ \ \varphi^0_{\pred{Void}}(x) \wedge \varphi^1_{\pred{Void}}(x)\\
\end{align*}
Then we let 
$$
\Phi_\mathrm{well} = 
\Phi^{\mathrm{funct}} \wedge 
\hspace{-3ex}\bigwedge_{\hspace{3ex}\pred{c}_k\in \Gamma,\,\pred{c} \in \mathrm{Cnst}}\hspace{-3ex} \Phi^{\mathrm{unique}}_{\pred{c}_k} \wedge 
\bigwedge_{\mathrm{Dec}\in \Gamma} \Phi_{\mathrm{Dec}}.
$$
%$$\Phi_{\mathrm{Dec}}
%    \bigwedge_{\pred{c}_k\in \Gamma} \Phi_{\pred{c}_k}
%    \bigwedge_{\pred{Add}_{\rpred,\vk} \in \Gamma} \Phi_{\pred{Add}_{\rpred,\vk}}
%    \bigwedge_{\pred{Recolor}_{k\to k'} \in \Gamma} \Phi_{k\to k'} \wedge
%    \Phi_{\oplus} \wedge
%    \Phi_{\pred{Void}} $$
